# Supplementary material for: Framework for Polarized Magnetic Neutron Scattering from Nanoparticle Assemblies with Vortex-Type Spin Textures
Source: arXiv:2404.15826 source file (2024-04-24)
Supplement: Supplementary file 1 [file MNS_VortexSpin_Supplemental.pdf]

# Supplemental Material to "Framework for Magnetic Neutron Scattering from Nanoparticle Assemblies with Vortex-Type Spin Textures"

Michael P. Adams,[1,*] Evelyn Pratami-Sinaga,[1] Štefan Liščák,[1] and Andreas Michels[1,†]

[1] *Department of Physics and Materials Science, University of Luxembourg, 162A Avenue de la Faiencerie, L-1511 Luxembourg, Grand Duchy of Luxembourg*

(Dated: April 24, 2024)

In this Supplemental Material we sketch the main ideas of the multi-nanoparticle power-series expansion (MNPSE) method that is used for the analytical calculation of the spin-flip SANS cross section, the chiral function, and the pair-distance distribution function. Moreover, the main expressions for the polarized SANS cross sections are displayed and details on the numerical micromagnetic simulations are furnished.

## I. SCATTERING GEOMETRY AND SPIN-FLIP SANS CROSS SECTION

The quantities of interest in the present paper are the elastic differential spin-flip scattering cross section and the related so-called chiral function, which are usually obtained in an uniaxial polarization-analysis experiment (e.g., [1–5]). For the most commonly used scattering geometry in magnetic SANS experiments (compare Fig. 1), where the applied magnetic field $\mathbf{H}_0 \parallel \mathbf{e}_z$ is perpendicular to the wave vector $\mathbf{k}_0 \parallel \mathbf{e}_x$ of the incident neutrons, the two spin-flip SANS cross sections $d\Sigma^{+-}_{\mathrm{sf}}/d\Omega$ and $d\Sigma^{-+}_{\mathrm{sf}}/d\Omega$ can be written as [6]:

$$\frac{d\Sigma^{+-}_{\mathrm{sf}}}{d\Omega} = \frac{8\pi^3}{V} b_{\mathrm{H}}^2 \left( |\widetilde{M}_x|^2 + |\widetilde{M}_y|^2 \cos^4\theta + |\widetilde{M}_z|^2 \sin^2\theta\cos^2\theta - (\widetilde{M}_y\widetilde{M}_z^* + \widetilde{M}_y^*\widetilde{M}_z)\sin\theta\cos^3\theta - i\chi \right), \quad (1)$$

$$\frac{d\Sigma^{-+}_{\mathrm{sf}}}{d\Omega} = \frac{8\pi^3}{V} b_{\mathrm{H}}^2 \left( |\widetilde{M}_x|^2 + |\widetilde{M}_y|^2 \cos^4\theta + |\widetilde{M}_z|^2 \sin^2\theta\cos^2\theta - (\widetilde{M}_y\widetilde{M}_z^* + \widetilde{M}_y^*\widetilde{M}_z)\sin\theta\cos^3\theta + i\chi \right). \quad (2)$$

The superscripts "+" and "−" refer to the neutron-spin orientation (parallel or antiparallel) relative to the direction of $\mathbf{H}_0$, $V$ denotes the scattering volume, $b_{\mathrm{H}} = 2.91 \times 10^8\,\mathrm{A}^{-1}\mathrm{m}^{-1}$ is the magnetic scattering length in the small-angle regime (the atomic magnetic form factor is approximated by 1, since we are dealing with forward scattering), $\widetilde{\mathbf{M}}(\mathbf{q}) = [\widetilde{M}_x(\mathbf{q}), \widetilde{M}_y(\mathbf{q}), \widetilde{M}_z(\mathbf{q})]$ represents the Fourier transform of the magnetization vector field $\mathbf{M}(\mathbf{r}) = [M_x(\mathbf{r}), M_y(\mathbf{r}), M_z(\mathbf{r})]$, $\theta$ denotes the angle between $\mathbf{q}$ and $\mathbf{H}_0$, the asterisk "$*$" marks the complex-conjugated quantity, $i^2 = -1$, and $\chi = \chi(\mathbf{q})$ is the chiral function. The latter quantity is obtained from (one-half times) the difference between the two spin-flip SANS cross sections, according to [6]:

$$\frac{d\Sigma_\chi}{d\Omega} = -iK\chi(\mathbf{q}) = \frac{1}{2}\left( \frac{d\Sigma^{+-}_{\mathrm{sf}}}{d\Omega} - \frac{d\Sigma^{-+}_{\mathrm{sf}}}{d\Omega} \right) = -iK \left[ (\widetilde{M}_x\widetilde{M}_y^* - \widetilde{M}_x^*\widetilde{M}_y)\cos^2\theta - (\widetilde{M}_x\widetilde{M}_z^* - \widetilde{M}_x^*\widetilde{M}_z)\sin\theta\cos\theta \right], \quad (3)$$

where $K = \frac{8\pi^3}{V} b_{\mathrm{H}}^2$. Note that the chiral function vanishes at complete magnetic saturation ($M_x^{H_0\to\infty} = M_y^{H_0\to\infty} = 0$) and for purely real-valued or for purely imaginary magnetization Fourier components $\widetilde{M}_{x,y,z}$.

Besides the difference between $d\Sigma^{+-}_{\mathrm{sf}}/d\Omega$ and $d\Sigma^{-+}_{\mathrm{sf}}/d\Omega$, we can also consider (one-half times) their sum:

$$\frac{d\Sigma_{\mathrm{sf}}}{d\Omega} = \frac{1}{2}\left( \frac{d\Sigma^{+-}_{\mathrm{sf}}}{d\Omega} + \frac{d\Sigma^{-+}_{\mathrm{sf}}}{d\Omega} \right) = K \left( |\widetilde{M}_x|^2 + |\widetilde{M}_y|^2 \cos^4\theta + |\widetilde{M}_z|^2 \sin^2\theta\cos^2\theta - (\widetilde{M}_y\widetilde{M}_z^* + \widetilde{M}_y^*\widetilde{M}_z)\sin\theta\cos^3\theta \right). \quad (4)$$

We note that the magnetization Fourier components are in general functions of $q$ and $\theta$, i.e., $\widetilde{M}_{x,y,z} = \widetilde{M}_{x,y,z}(q,\theta)$. The quantity $d\Sigma_{\mathrm{sf}}/d\Omega$ is called the (polarization-independent) spin-flip SANS cross section. The following symmetry relations hold for $d\Sigma_{\mathrm{sf}}/d\Omega$ (even under spatial inversion of $\mathbf{q}$) and $d\Sigma_\chi/d\Omega$ (odd under spatial inversion of $\mathbf{q}$):

$$\frac{d\Sigma_{\mathrm{sf}}}{d\Omega}(\mathbf{q}) = \frac{d\Sigma_{\mathrm{sf}}}{d\Omega}(-\mathbf{q}), \quad (5)$$

* Electronic address: michael.adams@uni.lu
† Electronic address: andreas.michels@uni.lu

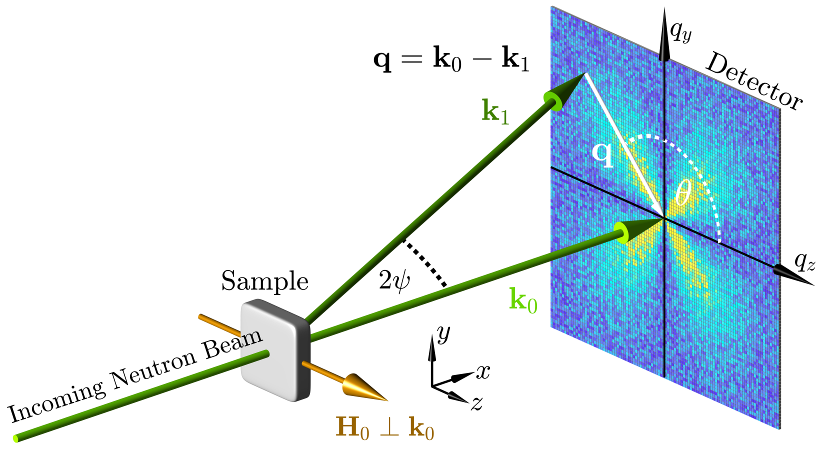


FIG. 1. Sketch of the neutron scattering geometry. The neutron optical elements (polarizer, spin flipper, analyzer) that are required to measure the spin-flip SANS cross section are not drawn. The applied magnetic field $\mathbf{H}_0 \parallel \mathbf{e}_z$ is perpendicular to the wave vector $\mathbf{k}_0 \parallel \mathbf{e}_x$ of the incident neutron beam ($\mathbf{H}_0 \perp \mathbf{k}_0$). The momentum-transfer or scattering vector $\mathbf{q}$ is defined as the difference between $\mathbf{k}_0$ and $\mathbf{k}_1$, i.e., $\mathbf{q} = \mathbf{k}_0 - \mathbf{k}_1$. SANS is usually implemented as elastic scattering ($k_0 = k_1 = 2\pi/\lambda$), and the component of $\mathbf{q}$ along the incident neutron beam, here $q_x$, is much smaller than the other two components so that $\mathbf{q} \cong [0, q_y, q_z] = q[0, \sin\theta, \cos\theta]$. This demonstrates that SANS probes predominantly correlations in the plane perpendicular to the incident beam. For elastic scattering, the magnitude of $\mathbf{q}$ is given by $q = (4\pi/\lambda)\sin(\psi)$, where $\lambda$ denotes the mean wavelength of the neutrons and $2\psi$ is the scattering angle. The angle $\theta = \angle(\mathbf{q}, \mathbf{H}_0)$ is used to describe the angular anisotropy of the recorded scattering pattern on the two-dimensional position-sensitive detector.

$$\frac{d\Sigma_\chi}{d\Omega}(\mathbf{q}) = -\frac{d\Sigma_\chi}{d\Omega}(-\mathbf{q}). \tag{6}$$

It is often convenient to average two-dimensional SANS data $f(\mathbf{q}) = f(q_y, q_z) = f(q, \theta)$, where $f$ either stands for $d\Sigma_{\mathrm{sf}}/d\Omega$ or for $d\Sigma_\chi/d\Omega$, along certain directions in $\mathbf{q}$ space, e.g. parallel ($\theta = 0$) or perpendicular ($\theta = \pi/2$) to the applied magnetic field, or even over the full angular $\theta$ range. In this paper, we consider $2\pi$ azimuthally-averaged SANS data

$$I_{\mathrm{sf}}(q) = \frac{1}{2\pi}\int_0^{2\pi} f(q,\theta)\, d\theta, \tag{7}$$

which allows for the computation of the pair-distance distribution function $p_{\mathrm{sf}}(r)$ according to

$$p_{\mathrm{sf}}(r) = r\int_0^\infty I_{\mathrm{sf}}(q)\sin(qr) q dq. \tag{8}$$

This Fourier transform corresponds to the distribution of real-space distances between volume elements inside the particle weighted by the excess scattering-length density distribution. As a reference for nonuniformly magnetized spherical particles, we specify here the $p_{\mathrm{sf}}(r)$ of a uniformly magnetized sphere, which for $r \leq D = 2R$ equals:

$$p_{\mathrm{sf}}(r) \propto r^2\left(1 - \frac{3r}{4R} + \frac{r^3}{16R^3}\right). \tag{9}$$

For the calculation of the spin-flip SANS cross section $d\Sigma_{\mathrm{sf}}/d\Omega$ [Eq. (4)] and the chiral function $d\Sigma_\chi/d\Omega$ [Eq. (3)], it is necessary to compute the discrete Fourier transform of all the $\mathbf{m}_i = \mathbf{m}_i(\mathbf{r})$ belonging to the spherical nanomagnet. Using $\boldsymbol{\mu}_i = \boldsymbol{\mu}_i(\mathbf{r}) = M_{\mathrm{s}} V_i \mathbf{m}_i(\mathbf{r})$, the discrete-space Fourier transform is computed as ($V_i = a^3$):

$$\widetilde{\mathbf{M}}(\mathbf{q}) \cong \frac{M_{\mathrm{s}} a^3 h(\mathbf{q})}{(2\pi)^{3/2}} \sum_{i=1}^{\mathcal{K}} \mathbf{m}_i \exp\left(-\mathrm{i}\mathbf{q}\cdot\mathbf{r}_i\right), \tag{10}$$

where $\mathbf{r}_i$ is the location point of the $i$th spin and $\mathbf{q}$ represents the wave vector (scattering vector). The function

$$h(\mathbf{q}) = \frac{\sin(q_x a/2)}{q_x a/2}\frac{\sin(q_y a/2)}{q_y a/2}\frac{\sin(q_z a/2)}{q_z a/2} \tag{11}$$

denotes the form factor of the cubic discretization cell with $a = 2\,\mathrm{nm}$ being the cell size; for $|q_{x,y,z}|a/2 \ll 1$, $h \rightarrow 1$. For atomistic calculation [7, 8], this correction is irrelevant in the small-angle regime, but for the present calculation, the cell size becomes already noticeable for $q \gtrsim 0.3\,\mathrm{nm}^{-1}$. Equation (10) establishes the relation between the outcome of the simulations, $\mathbf{m}_i$, and $d\Sigma_{\mathrm{sf}}/d\Omega$ and $d\Sigma_{\chi}/d\Omega$. The Fourier components are evaluated in the plane $q_x = 0$ (corresponding to the scattering geometry shown in Fig. 1 with $\mathbf{q} \cong [0, q_y, q_z] = q[0, \sin\theta, \cos\theta]$) and used in Eqs. (3) and (4) to compute the spin-flip SANS cross section and the chiral function.

## II. DETAILS ON THE MICROMAGNETIC SIMULATIONS

We were using the open-source software package Mumax3 (version 3.10) for the micromagnetic simulations [9, 10]. This program is a widely used micromagnetic simulation tool that enables researchers to investigate the static and dynamic nanoscale behavior of magnetic materials. Mumax3 employs a finite-difference discretization scheme of space using an orthorhombic grid of cells. The following contributions to the total magnetic Gibbs free energy $G = E_{\mathrm{z}} + E_{\mathrm{d}} + E_{\mathrm{ani}} + E_{\mathrm{ex}}$ were taken into account: Zeeman energy $E_{\mathrm{z}}$ in the external magnetic field, dipolar (magnetostatic) interaction energy $E_{\mathrm{d}}$, energy of the (cubic) magnetocrystalline anisotropy $E_{\mathrm{ani}}$, and the isotropic and symmetric exchange energy $E_{\mathrm{ex}}$. The continuum expressions for these energies are the following [11]:

$$E_{\mathrm{z}} = -\mu_0 M_{\mathrm{s}} \int \mathbf{m} \cdot \mathbf{H}_0 \, dV, \tag{12}$$

$$E_{\mathrm{d}} = -\frac{1}{2}\mu_0 M_{\mathrm{s}} \int \mathbf{m} \cdot \mathbf{H}_{\mathrm{d}} \, dV, \tag{13}$$

$$E_{\mathrm{ani}} = K_{\mathrm{c1}} \int \left[ (\mathbf{c}_1 \cdot \mathbf{m})^2 (\mathbf{c}_2 \cdot \mathbf{m})^2 + (\mathbf{c}_1 \cdot \mathbf{m})^2 (\mathbf{c}_3 \cdot \mathbf{m})^2 + (\mathbf{c}_2 \cdot \mathbf{m})^2 (\mathbf{c}_3 \cdot \mathbf{m})^2 \right] dV, \tag{14}$$

$$E_{\mathrm{ex}} = A \int \left[ (\nabla m_x)^2 + (\nabla m_y)^2 + (\nabla m_z)^2 \right] \, dV, \tag{15}$$

where $\mu_0 = 4\pi \times 10^{-7}\,\mathrm{Tm/A}$, $\mathbf{m}(\mathbf{r}) = \mathbf{M}(\mathbf{r})/M_{\mathrm{s}}$ denotes the unit magnetization vector field with $M_{\mathrm{s}}$ being the saturation magnetization, $\mathbf{H}_0$ is the (constant) applied magnetic field, $\mathbf{H}_{\mathrm{d}} = \mathbf{H}_{\mathrm{d}}(\mathbf{r}; \mathbf{M}(\mathbf{r}))$ is the magnetostatic self-interaction field, $K_{\mathrm{c1}}$ is the first-order cubic anisotropy constant with the $\mathbf{c}_{1,2,3}$ vectors representing the local (mutually perpendicular) cubic anisotropy axes [12], $A$ is the exchange-stiffness constant, and the integrals are taken over the volume of the sample. In the simulations, we used the following material parameters for iron: $M_{\mathrm{s}} = 1700\,\mathrm{kA/m}$, $K_{\mathrm{c1}} = +4.7 \times 10^4\,\mathrm{J/m^3}$, and $A = 1.0 \times 10^{-11}\,\mathrm{J/m}$. These values result in a magnetostatic exchange length of $l_{\mathrm{s}} = \sqrt{2A/(\mu_0 M_{\mathrm{s}}^2)} = 2.3\,\mathrm{nm}$ and in a domain-wall parameter of $l_{\mathrm{k}} = \sqrt{A/K_{\mathrm{c1}}} = 14.6\,\mathrm{nm}$. We refer to Ref. [9] for a discussion of how the above continuum expressions for the magnetic energies are numerically implemented on a discrete spatial grid.

We carried out simulations for a sphere diameter of $D = 40\,\mathrm{nm}$. The sphere volume was discretized into cubical cells "$i$" with a size (volume) of $V_i = 2 \times 2 \times 2\ \mathrm{nm}^3$ (finite-difference method). This cell size is motivated by the above values for $l_{\mathrm{s}}$ and $l_{\mathrm{k}}$ and by the aim to resolve spatial variations in the magnetization that are smaller than these characteristic length scales. In each cell "$i$" with volume $V_i$, the magnetic moment vector is given by $\boldsymbol{\mu}_i = \boldsymbol{\mu}_i(\mathbf{r}) = M_{\mathrm{s}} V_i \mathbf{m}_i(\mathbf{r})$, where $\mathbf{m}_i(\mathbf{r})$ is a unit vector along the local direction of the magnetization. Open boundary conditions were used. We are interested in the scattering behavior of an ensemble of noninteracting particles having random easy-axis orientations; 800 random orientations between the cubic anisotropy axes and $\mathbf{H}_0$ were used to compute randomly-averaged quantities. All simulations were carried out by first saturating the nanoparticle by a strong external field $\mathbf{H}_0$, and then the field was decreased in steps of typically $5\,\mathrm{mT}$ following the major hysteresis loop. For each step of $H_0$ and for each particular easy-axis orientation, we have obtained the equilibrium spin structure $m_{x,y,z}(x, y, z)$ by employing both the "Relax" and "Minimize" functions of Mumax3. The former solves the Landau-Lifshitz-Gilbert equation without the precessional term and the latter uses the conjugate-gradient method to find the configuration of minimum energy.

Using the results of the Mumax3 simulations, we determine the vortex rotation axis vector $\mathbf{a}$ of a particular magnetization structure by employing a linear least-squares method. For this analysis, we assume the following linear magnetization function:

$$\mathbf{m}_{\mathrm{lin}}(\mathbf{r}) = \begin{bmatrix} m_0^x \\ m_0^y \\ m_0^z \end{bmatrix} + \begin{bmatrix} m_1^{xx} & m_1^{xy} & m_1^{xz} \\ m_1^{yx} & m_1^{yy} & m_1^{yz} \\ m_1^{zx} & m_1^{zy} & m_1^{zz} \end{bmatrix} \cdot \begin{bmatrix} x \\ y \\ z \end{bmatrix}, \tag{16}$$

and minimize the following mean-square-error function:

$$\epsilon = \frac{1}{n}\sum_{k=1}^{n} \|\mathbf{m}_k - \mathbf{m}_{\mathrm{lin}}(\mathbf{r}_k)\|^2, \tag{17}$$

where $\mathbf{m}_k$ is the magnetization vector of the simulation cell "$k$", $\mathbf{r}_k$ is the corresponding position vector, and $n$ denotes the number of discretization cells of an individual particle. The minimization of $\epsilon$ is achieved by solving the following system of linear equations (with $\kappa \in \{x, y, z\}$):

$$\mathbf{A}\mathbf{x}_\kappa = \mathbf{v}_\kappa, \tag{18}$$

with the system matrix

$$\mathbf{A} = \sum_{k=1}^{n} \begin{bmatrix} 1 & \mathbf{r}_k^T \\ \mathbf{r}_k & \mathbf{r}_k \otimes \mathbf{r}_k \end{bmatrix}, \tag{19}$$

the coefficient vector

$$\mathbf{x}_\kappa = \begin{bmatrix} m_0^\kappa & m_1^{\kappa x} & m_1^{\kappa y} & m_1^{\kappa z} \end{bmatrix}^T, \tag{20}$$

and the constant vector

$$\mathbf{v}_\kappa = \sum_{k=1}^{n} \begin{bmatrix} m_k^\kappa \\ m_k^\kappa \mathbf{r}_k \end{bmatrix}. \tag{21}$$

The normalized rotation axis vector $\mathbf{a}$ is then computed from the curl of the linear magnetization function [Eq. (16)] as follows

$$\mathbf{a} = \frac{\nabla \times \mathbf{m}_{\mathrm{lin}}}{\|\nabla \times \mathbf{m}_{\mathrm{lin}}\|} = \frac{[m_1^{zy} - m_1^{yz},\ m_1^{xz} - m_1^{zx},\ m_1^{yx} - m_1^{xy}]}{\sqrt{(m_1^{zy} - m_1^{yz})^2 + (m_1^{xz} - m_1^{zx})^2 + (m_1^{yx} - m_1^{xy})^2}}. \tag{22}$$

In the fully saturated state, the vector $\mathbf{a}$ does not exist since the magnetization is uniform.

Figure 2 displays micromagnetic simulation data for the vortex profile in the remanent state. It is seen that the radial component $m_\rho$ is equal to zero over the particle radius (on the average), while the tangential component $m_\beta$ increases to unity (due to flux closure), and the magnetization component $m_z$ decreases from about unity at the sphere center to a slightly negative but constant value at the radius. Figure 8 shows the corresponding results for a uniaxial particle anisotropy (Fig. 2 is for a cubic particle anisotropy).

The vortex-axes distribution function $\psi(\alpha, \beta)$, for use in Eq. (74) to compute the spin-flip SANS cross section and chiral function, is extracted from the Mumax3 simulation data using the following recipe: (i) We assume a given set of nonzero random vectors $\mathbf{m}^k = [m_x^k, m_y^k, m_z^k]$ with $k = \{1, 2, 3, ..., K\}$. These random vectors are represented by either the easy axes of the particles, their net magnetizations, or their vortex axes [see Fig. 3(a,b,c)]. (ii) We compute the corresponding set of spherical angles

$$\alpha^k = \mathrm{arctan2}\left(\sqrt{(m_x^k)^2 + (m_y^k)^2}, m_z^k\right), \tag{23}$$

$$\beta^k = \mathrm{arctan2}\left(m_y^k, m_x^k\right), \tag{24}$$

which are plotted in Fig. 3(d,e,f). (iii) We define a rectangular grid

$$\alpha_\mu = h\mu + h/2, \qquad \mu = \{0, 1, 2, ..., N-1\}, \tag{25}$$

$$\beta_\nu = h\nu + h/2, \qquad \nu = \{0, 1, 2, ..., 2N-1\}, \tag{26}$$

where $h = \pi/N$ is the step size (the grid consists of $N \times 2N$ squares of side length $h$, where the $(\alpha_\mu, \beta_\nu)$ are the center points of the squares). (iv) From the data set $(\alpha^k, \beta^k)$ we compute the empirical probability $P_{\mu\nu}$ corresponding to the binning $(\alpha_\mu, \beta_\nu)$:

$$P_{\mu\nu} = \frac{1}{K}\sum_{k=1}^{K} \delta_{\mu\nu}(\alpha^k, \beta^k), \tag{27}$$

$$\delta_{\mu\nu}(\alpha^k, \beta^k) = \begin{cases} 1 & , \text{ if } (-h/2 < \alpha^k - \alpha_\mu < h/2) \wedge (-h/2 < \beta^k - \beta_\nu < h/2) \\ 0 & , \text{ else} \end{cases}. \tag{28}$$

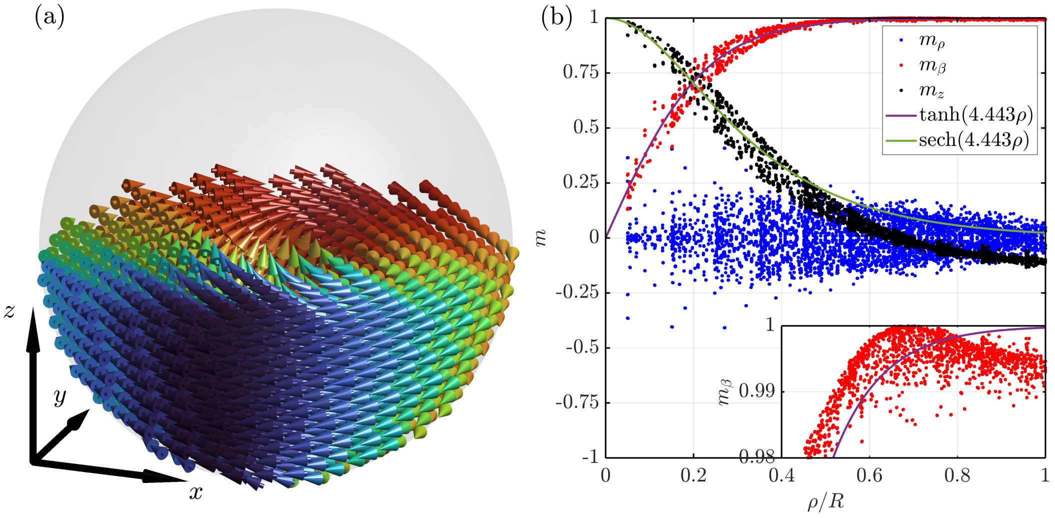


FIG. 2. (a) Example for a real-space spin structure in the remanent state ($B_0 = 0\,\mathrm{T}$). (b) Vortex profile in the remanent state. The data points represent the collective magnetization data of 10 nanoparticles with 4224 magnetic moments each with reference to their individual vortex reference frame. The orientation of the cubic anisotropy varies randomly from particle to particle (particle size is 40 nm, discretized into $2 \times 2 \times 2\ \mathrm{nm}^3$). Initially all structures were saturated by a strong applied field $\mathbf{H}_0 \parallel \mathbf{e}_z$. The cylindrical components of the magnetization, $m_\rho, m_\beta, m_z$, are represented as a function of the cylinder radius $\rho = \sqrt{x^2 + y^2}$ and follow the constraint that $m_\rho^2 + m_\beta^2 + m_z^2 = 1$. The azimuthal component $m_\beta$ and the axial component $m_z$ approximately follow hyperbolic tangent and secant functions, respectively.

The summation over the $P_{\mu\nu}$ is equal to unity:

$$\sum_{\mu=0}^{N-1} \sum_{\nu=0}^{2N-1} P_{\mu\nu} = 1. \tag{29}$$

(v) By normalizing the empirical probability, we estimate the spherical probability distribution $\psi_{\mu\nu}$ as follows:

$$\psi(\alpha_\mu, \beta_\nu) \approx \psi_{\mu\nu} = \frac{P_{\mu\nu}}{h^2 \sin(\alpha_\mu)}, \qquad \left[\text{spherical normalization } \int_0^{2\pi} \int_0^{\pi} \psi(\alpha, \beta) \sin\alpha \, d\alpha d\beta = 1\right]. \tag{30}$$

(vi) By assuming azimuthal symmetry, we can improve the statistics by averaging (integration using the trapezoidal rule) and rescaling by the factor $(2\pi)^{-1}$:

$$\psi(\alpha, \beta) \approx \psi_\mu = \frac{1}{2\pi} \frac{h}{2} \sum_{\nu=0}^{2N-2} (\psi_{\mu,\nu} + \psi_{\mu,\nu+1}), \qquad \left[\text{azimuthal symmetry: } \psi(\alpha, \beta) = \frac{1}{2\pi} \int_0^{2\pi} \psi(\alpha, \beta) d\beta\right] \tag{31}$$

(vii) The resulting numbers $\psi_\mu$ are displayed in Fig. 3(g,h,i). In Fig. 3(g) we show that, for the case of a uniform distribution on the spherical surface, the probability distribution function $\psi(\alpha, \beta) = (4\pi)^{-1}$. This result is reasonable due to the spherical normalization foe the probability distribution function $\psi$.

## III. MULTI-NANOPARTICLE POWER-SERIES EXPANSION (MNPSE) METHOD FOR THE POLARIZED SANS CROSS SECTION

For the sake of self-contained presentation, we repeat here the main steps of the MNPSE approach [8].

### A. Magnetization power-series expansion, Fourier cross-correlation matrix, and spin-flip SANS cross section

We consider an ensemble of magnetic nanoparticles rigidly embedded in a nonmagnetic and homogeneous matrix. The global magnetization vector field of the system, $\mathbf{M}(\mathbf{r}) = [M^x(\mathbf{r}), M^y(\mathbf{r}), M^z(\mathbf{r})]$, is generally a discontinuous

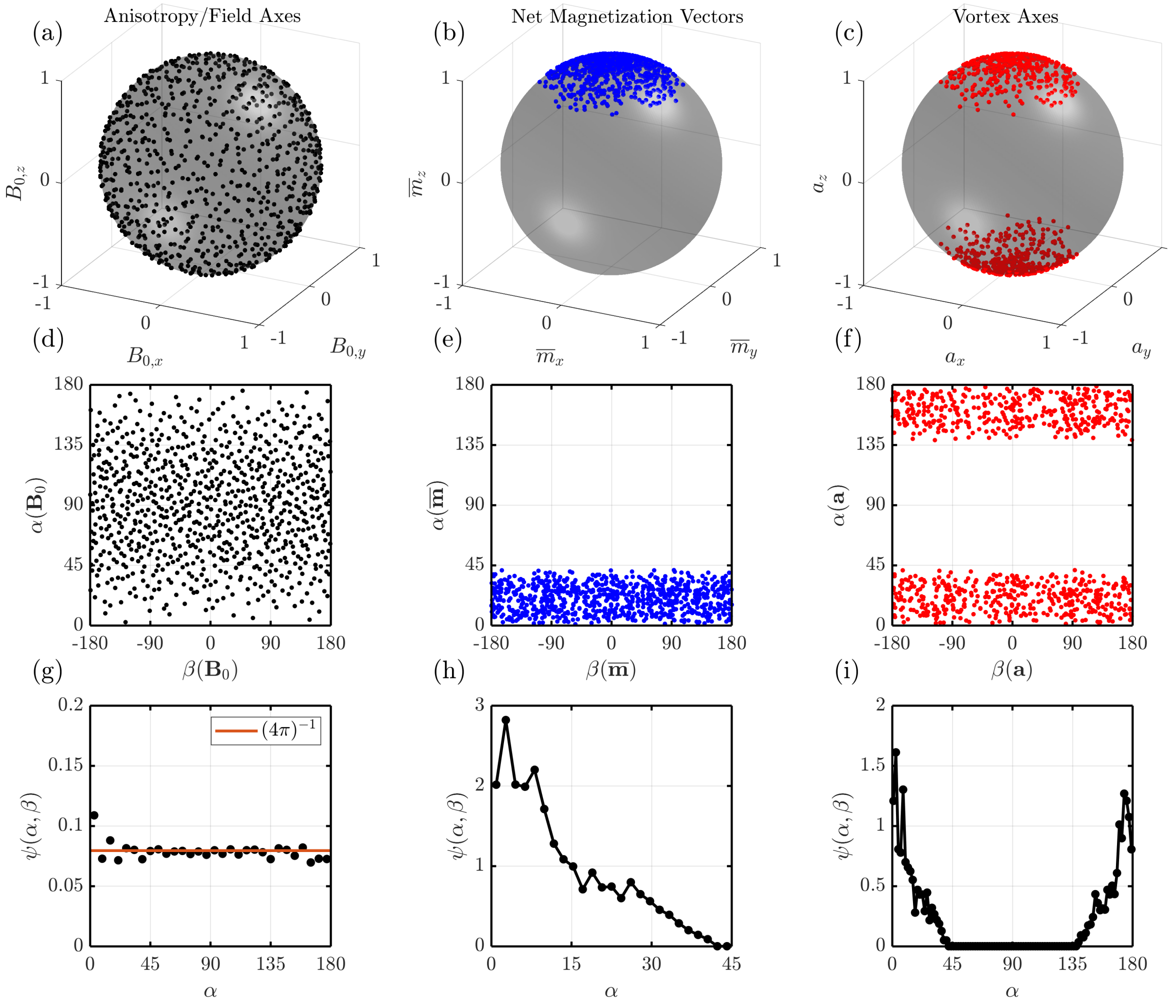


FIG. 3. Distribution of (a) the cubic anisotropy axes/applied fields, (b) the net (average) magnetization vectors, and (c) the vortex rotation axes vectors on the unit sphere at remanence. Initially all structures were saturated by a strong applied field $\mathbf{H}_0 \parallel \mathbf{e}_z$. Data of 800 particles with random cubic anisotropy are shown. $\alpha$ and $\beta$ in (d,e,f) denote the respective polar and azimuthal angles [computed according to Eqs. (23) and (24)]. The anisotropy axes are randomly distributed over the whole unit sphere and follow a $\psi(\alpha,\beta) = (4\pi)^{-1}$ distribution function (g). The net magnetization vectors at remanence, $\overline{\mathbf{m}}$, are azimuthally-symmetric ($\beta$ independent) and bound by $\alpha \lesssim 45^\circ$ (h). The uniaxial vortex rotation axes $\mathbf{a}$ are symmetrically bound by $0^\circ \lesssim \alpha \lesssim 45^\circ$ and $135^\circ \lesssim \alpha \lesssim 180^\circ$ and (for $\alpha \lesssim \alpha_c = 45^\circ$) approximately follow a $\psi(\alpha,\beta) = \Theta(1-\alpha/\alpha_c)/[2\pi(1-\cos\alpha_c)]$ distribution (i). The vortex axes in the upper hemisphere ($\alpha < 90^\circ$) correspond to a mathematically positive rotation in the $xy$ plane and vice versa for the lower hemisphere ($\alpha > 90^\circ$).

function, since $\mathbf{M}$ vanishes in the space between the particles; $\mathbf{r} = [x, y, z]$ is the position vector in the laboratory frame. For the formulation of this discontinuous behavior, we use the indicator function (or particle shape function with particle index $\nu$)

$$S_\nu(\mathbf{r}'_\nu) = \begin{cases} 1 & , \ \mathbf{r}'_\nu \in V'_\nu \\ 0 & , \ \mathbf{r}'_\nu \notin V'_\nu \end{cases}, \tag{32}$$

where $V'_\nu \subset \mathbb{R}^3$ denotes the set of points within the $\nu$-th particle volume with reference to the local particle frame, and $\mathbf{r}'_\nu = [x'_\nu, y'_\nu, z'_\nu]$ represent the local coordinates (see Fig. 4). The transformation between the global point set $V_\nu$ and the local point set $V'_\nu$ is then obtained by $V'_\nu = \{\mathbf{r} - \mathbf{a}_\nu : \mathbf{r} \in V_\nu\}$ (with the inverse transformation: $V_\nu = \{\mathbf{r}'_\nu + \mathbf{a}_\nu : \mathbf{r}'_\nu \in V'_\nu\}$), where $\mathbf{a}_\nu = [a^x_\nu, a^y_\nu, a^z_\nu]$ is a constant shift vector that points from the origin of the global $\mathbf{r}$ coordinate system to the origin of the local $\mathbf{r}'_\nu$ system. The corresponding linear coordinate transformation is then given by $\mathbf{r}'_\nu = \mathbf{r} - \mathbf{a}_\nu$, while the volume $v_\nu$ of the $\nu$-th particle is obtained via integration of the corresponding shape

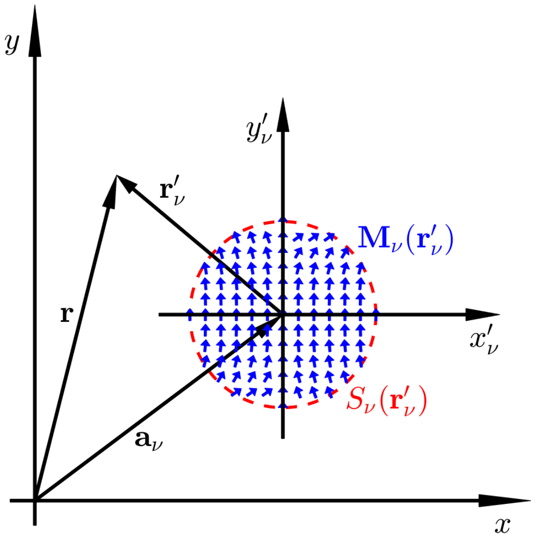


FIG. 4. Sketch illustrating the relationship between the global unprimed ($\mathbf{r}$) laboratory coordinate system and the local primed ($\mathbf{r}'_\nu$) system of particle $\nu$ with magnetization $\mathbf{M}_\nu(\mathbf{r}'_\nu)$ and shape function $S_\nu(\mathbf{r}'_\nu)$. $\mathbf{a}_\nu$ is a constant shift vector that points from the origin of the global $\mathbf{r}$ coordinate system to the origin of the local $\mathbf{r}'_\nu$ system. For simplicity, the $z$ coordinate specifying the third space dimension has been ignored.

function:

$$v_\nu = \int_{\mathbb{R}^3} S_\nu(\mathbf{r}'_\nu) d^3 r'_\nu. \tag{33}$$

To account for an inhomogeneous magnetic microstructure, we describe the Cartesian magnetization vector field components $M^\mu_\nu$ (with $\mu \in \{x, y, z\}$) for the $\nu$-th particle as the product of its shape function and a power series:

$$M^\mu_\nu(\mathbf{r}'_\nu) = S_\nu(\mathbf{r}'_\nu) \sum_{k,m,n=0}^{\infty} M^\mu_{\nu,(k,m,n)} x'^k_\nu y'^m_\nu z'^n_\nu, \tag{34}$$

where $M^\mu_{\nu,(k,m,n)}$ are arbitrary constant expansion coefficients, which may depend on temperature, applied magnetic field, and the type of material. The global Cartesian magnetization vector field components $M^\mu$ then follow as the sum over the individual magnetization components $M^\mu_\nu$ shifted by $\mathbf{a}_\nu$:

$$\begin{aligned} M^\mu(\mathbf{r}) &= \sum_{\nu=1}^{\mathcal{K}} M^\mu_\nu(\mathbf{r} - \mathbf{a}_\nu) \\ &= \sum_{\nu=1}^{\mathcal{K}} \left[ S_\nu(\mathbf{r} - \mathbf{a}_\nu) \sum_{k,m,n=0}^{\infty} M^\mu_{\nu,(k,m,n)} (x - a^x_\nu)^k (y - a^y_\nu)^m (z - a^z_\nu)^n \right], \end{aligned} \tag{35}$$

$\mathcal{K}$ being the number of particles in the assembly. For the further derivations, we prefer the Einstein and multi-index notation. Using these notation concepts, Eq. (35) reads:

$$M^\mu(\mathbf{r}) = S_\nu(\mathbf{r} - \mathbf{a}_\nu) M^\mu_{\nu,\boldsymbol{\alpha}} (\mathbf{r} - \mathbf{a}_\nu)^{\boldsymbol{\alpha}}, \tag{36}$$

where $\boldsymbol{\alpha} = (k, m, n)$ represents a multi-index. The zero-order case of $\boldsymbol{\alpha} = (0, 0, 0)$ corresponds to the situation of an ensemble of uniformly magnetized nanoparticles. Higher-order terms in this series take into account the local spatial nonuniformities in $\mathbf{M}$.

For the computation of the magnetic SANS cross section, the next step is to perform the spatial Fourier transform

$$\widetilde{M}^\mu(\mathbf{q}) = \frac{1}{(2\pi)^{3/2}} \int_{\mathbb{R}^3} M^\mu(\mathbf{r}) \exp(-i\mathbf{q} \cdot \mathbf{r}) d^3 r. \tag{37}$$

Instead of direct integration, we can use the shift and derivation theorem of Fourier theory, such that the Fourier transform of Eq. (36) can be expressed as

$$\widetilde{M}^{\mu}(\mathbf{q}) = i^{|\boldsymbol{\alpha}|} M^{\mu}_{\nu,\boldsymbol{\alpha}} \exp(-\mathrm{i}\mathbf{q}\cdot\mathbf{a}_{\nu}) \partial^{\boldsymbol{\alpha}} \widetilde{S}_{\nu}(\mathbf{q}), \tag{38}$$

where $i$ is the imaginary number ($i^2 = -1$).

In the sequel, the derivative $\partial^{\boldsymbol{\alpha}}$, with $\boldsymbol{\alpha} = (k, m, n)$, will denote the $|\boldsymbol{\alpha}|$-th order mixed partial derivative

$$\partial^{\boldsymbol{\alpha}} \equiv \frac{\partial^k}{\partial q_x^k} \frac{\partial^m}{\partial q_y^m} \frac{\partial^n}{\partial q_z^n}, \tag{39}$$

with $|\boldsymbol{\alpha}| = k + m + n$ being the sum of components of the multi-index $\boldsymbol{\alpha} = (k, m, n)$. Likewise, the compact sum $\sum_{\boldsymbol{\alpha}}$ should be understood as the triple sum $\sum_k \sum_m \sum_n$. $\widetilde{S}_{\nu}(\mathbf{q})$ is the Fourier transform of the indicator function defined by

$$\widetilde{S}_{\nu}(\mathbf{q}) = \frac{1}{(2\pi)^{3/2}} \int_{\mathbb{R}^3} S_{\nu}(\mathbf{r}) \exp(-\mathrm{i}\mathbf{q}\cdot\mathbf{r}) d^3 r. \tag{40}$$

Next, introducing the following Fourier cross-correlation functions $\widetilde{\Gamma}^{\iota\kappa} : \mathbb{R}^3 \to \mathbb{C}$ with $\iota, \kappa \in \{x, y, z\}$ ("$*$" stands for the complex conjugate),

$$\begin{aligned} \widetilde{\Gamma}^{\iota\kappa}(\mathbf{q}) &= \left[\widetilde{M}^{\iota}(\mathbf{q})\right] \left[\widetilde{M}^{\kappa}(\mathbf{q})\right]^* \\ &= i^{|\boldsymbol{\alpha}|-|\boldsymbol{\beta}|} M^{\iota}_{\nu,\boldsymbol{\alpha}} M^{\kappa}_{\mu,\boldsymbol{\beta}} \exp(-\mathrm{i}\mathbf{q}\cdot[\mathbf{a}_{\nu} - \mathbf{a}_{\mu}]) \partial^{\boldsymbol{\alpha}} \widetilde{S}_{\nu}(\mathbf{q}) \partial^{\boldsymbol{\beta}} \widetilde{S}^*_{\mu}(\mathbf{q}), \end{aligned} \tag{41}$$

we rewrite the spin-flip SANS cross section for the perpendicular scattering geometry [see Fig. 1 and Eq. (4)] as follows:

$$\frac{d\Sigma_{\mathrm{sf}}}{d\Omega}(\mathbf{q}) = K \left( \widetilde{\Gamma}^{xx} + \widetilde{\Gamma}^{yy} \cos^4\theta + \widetilde{\Gamma}^{zz} \sin^2\theta \cos^2\theta - [\widetilde{\Gamma}^{yz} + \widetilde{\Gamma}^{zy}] \sin\theta \cos^3\theta \right), \tag{42}$$

with $\mathbf{q} = q[0, \sin\theta, \cos\theta]$. We emphasize that the $\widetilde{\Gamma}^{\iota\kappa}$ are functions of $q$ and $\theta$. In the following discussion, we focus on the first-order approximation and we neglect interparticle interaction effects.

### B. First-order approximation for a dilute ensemble of spherical nanoparticles

For a dilute ($\mathbf{a}_{\nu} = \mathbf{a}_{\mu}$) and monodisperse ($\widetilde{S}_{\nu} = \widetilde{S}_{\mu} = \widetilde{S}$) ensemble of spherical nanoparticles (with radius $R$), the Fourier cross-correlation functions simplify to [6]:

$$\widetilde{\Gamma}^{\iota\kappa}(\mathbf{q}) = i^{|\boldsymbol{\alpha}|-|\boldsymbol{\beta}|} M^{\iota}_{\mu,\boldsymbol{\alpha}} M^{\kappa}_{\mu,\boldsymbol{\beta}} \partial^{\boldsymbol{\alpha}} \widetilde{S}(q) \partial^{\boldsymbol{\beta}} \widetilde{S}(q), \tag{43}$$

where $q = \sqrt{q_x^2 + q_y^2 + q_z^2}$, and

$$\widetilde{S}(q) = \frac{3V_{\mathrm{s}}}{(2\pi)^{3/2}} \frac{j_1(qR)}{qR} \quad \text{with} \quad V_{\mathrm{s}} = \frac{4\pi R^3}{3}. \tag{44}$$

$j_1(u) = \sin u/u^2 - \cos u/u$ is the first-order spherical Bessel function. In this special case of spherical nanoparticles (where $\widetilde{S} = \widetilde{S}^*$), the Fourier transform of the indicator function becomes real-valued, such that it is obvious that only terms with $|\boldsymbol{\alpha}| - |\boldsymbol{\beta}| = 2u$ (with $u \in \mathbb{Z}$) contribute to Eq. (43) [13]. In the study of Adams et. al. [14], the zero-order case of Eq. (43), which reflects a dilute and monodisperse ensemble of uniformly magnetized spherical nanoparticles, was studied in the context of the Stoner-Wohlfarth model. In this situation, the cross-correlation matrix can be written as:

$$\widetilde{\Gamma}^{\iota\kappa}(\mathbf{q}) = \Gamma_0^{\iota\kappa} [\widetilde{S}(q)]^2 \quad \text{with} \quad \Gamma_0^{\iota\kappa} = M^{\iota}_{\nu,(0,0,0)} M^{\kappa}_{\nu,(0,0,0)}. \tag{45}$$

The real-space cross-correlation matrix $\Gamma_0^{\iota\kappa}$ is a function of the applied magnetic field, such that the two-dimensional magnetic SANS cross section exhibits different types of angular anisotropies, even for randomly-averaged ensembles at remanence or at the coercive field [14].

Now, taking into account spin inhomogeneities up to the first polynomial order in the expansion of the magnetization [Eq. (36)], Eq. (43) becomes:

$$\widetilde{\Gamma}^{\iota\kappa}(\mathbf{q}) = \Gamma_0^{\iota\kappa}\widetilde{S}^2 + \Gamma_{1,lm}^{\iota\kappa}\left[\frac{\partial\widetilde{S}}{\partial q_l}\right]\left[\frac{\partial\widetilde{S}}{\partial q_m}\right], \tag{46}$$

where we have defined the combinations of polynomial magnetization coefficients as:

$$\Gamma_0^{\iota\kappa} = M^{\iota}_{\nu,\boldsymbol{F}_0}M^{\kappa}_{\nu,\boldsymbol{F}_0}, \tag{47}$$
$$\Gamma_{1,\ell m}^{\iota\kappa} = M^{\iota}_{\nu,\boldsymbol{F}_\ell}M^{\kappa}_{\nu,\boldsymbol{F}_m}, \tag{48}$$

and we use the following $\boldsymbol{F}_i$ symbol for booking the multi-indices of the magnetization coefficients:

$$\boldsymbol{F}_i = \begin{cases} (0,0,0) & , i=0 \\ (1,0,0) & , i=x \\ (0,1,0) & , i=y \\ (0,0,1) & , i=z \end{cases}. \tag{49}$$

We note that the new $\Gamma$ and $C$ coefficients include the sum over the ensemble of nanoparticles. This is seen from the fact that the index $\nu$ occurs only on the right-hand-side of Eqs. (47) and (48), but not on the left-hand-side. Since (for a spherical particle) the Fourier transform of the indicator function $\widetilde{S}$ depends only $q = \sqrt{q_x^2 + q_y^2 + q_z^2}$, we can express the partial derivatives of $\widetilde{S}$ in Eq. (46) (using the chain rule) up to the first-order as:

$$\widetilde{S}(q) = \frac{3V_{\rm s}}{(2\pi)^{3/2}}\frac{j_1(qR)}{qR}, \qquad \frac{\partial\widetilde{S}}{\partial q_\alpha} = \hat{q}_\alpha\widetilde{S}' \tag{50}$$

where $\hat{q}_l = q_l/q$ (with $l = x, y, z$), $\delta^{\alpha\beta}$ is the Kronecker delta symbol, and the prime denotes the derivative with respect to the radial coordinate, i.e., $\widetilde{S}' = d\widetilde{S}/dq$ and $\widetilde{S}'' = d^2\widetilde{S}/dq^2$. Using the results from Eq. (50), we can rewrite Eq. (46) as follows:

$$\widetilde{\Gamma}^{\iota\kappa}(\mathbf{q}) = \Gamma_0^{\iota\kappa}\widetilde{S}^2 + \Gamma_{1,\ell m}^{\iota\kappa}\hat{q}^\ell\hat{q}^m\widetilde{S}'^2. \tag{51}$$

In the above formulation, we see that the angular ($\hat{q}_\alpha$) dependence and the radial ($q$) dependence of the cross-correlation functions are separated in the sense of a multiplication. This is an important property that facilitates the further calculations, especially the azimuthal averaging of the magnetic SANS cross section (see below). Furthermore, inspection of Eq. (50) shows that the shape function $\widetilde{S}$ and its ordinary derivatives with respect to the radial coordinate $q$ also depend on the radius $R$ of the particle. Therefore, it is convenient to define the dimensionless function $f(u = qR)$ such that the shape function $\widetilde{S}$ and its derivatives can be written as follows:

$$f(u) = \frac{j_1(u)}{u} = \frac{\sin u - u\cos u}{u^3}, \qquad \widetilde{S}(q) = \frac{3V_{\rm s}}{(2\pi)^{3/2}}f(qR), \tag{52}$$
$$f'(u) = \frac{(u^2-3)\sin u + 3u\cos u}{u^4}, \qquad \widetilde{S}'(q) = \frac{3V_{\rm s}R}{(2\pi)^{3/2}}f'(qR). \tag{53}$$

In order to write the cross-correlation matrix [Eq. (51)] in compact form, we introduce the following radial functions $g_k$ and angular functions $G_k^{\iota\kappa}$:

$$g_0(u) = (f(u))^2, \qquad G_0^{\iota\kappa}(\hat{\mathbf{q}}) = h\Gamma_0^{\iota\kappa}, \tag{54}$$
$$g_1(u) = (f'(u))^2, \qquad G_1^{\iota\kappa}(\hat{\mathbf{q}}) = hR^2\Gamma_{1,\ell m}^{\iota\kappa}\hat{q}^\ell\hat{q}^m, \tag{55}$$

The functions $g_0(u)$ and $g_1(u)$ are shown in Fig. 5. For completeness we provide the limit of the functions $g_i(u)$ for $u \to 0$:

$$\lim_{u\to 0} g_0(u) = \frac{1}{9} \qquad \lim_{u\to 0} g_1(u) = 0. \tag{56}$$

The azimuthally-averaged spin-flip SANS cross section $I_{\rm sf}(q)$ for the perpendicular scattering geometry is then obtained by a projection onto the two-dimensional detector plane, i.e., setting $\hat{\mathbf{q}} = [0, \sin\theta, \cos\theta]$ in Eq. (51). Substituting

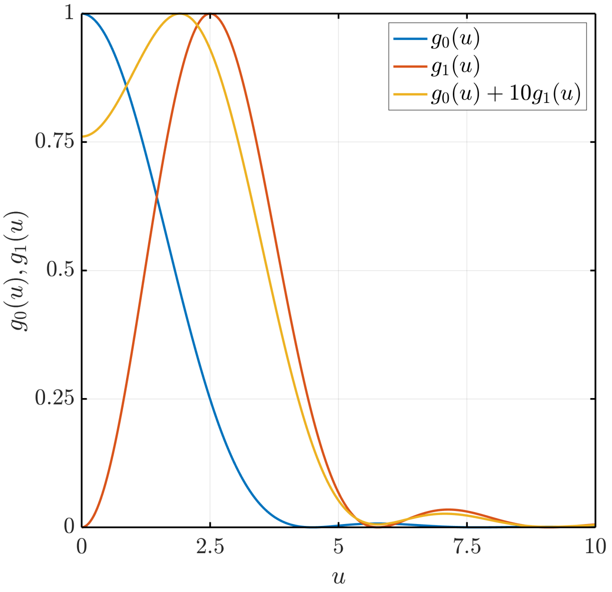


FIG. 5. The functions $g_0(u)$, $g_1(u)$, and their weighted sum. The functions are normalized to their maximum values.

Eq. (51) for the $\widetilde{\Gamma}^{\iota\kappa}(\mathbf{q})$ into Eq. (72) and carrying out an azimuthal average $[(2\pi)^{-1}\int_0^{2\pi}(...)d\theta]$, we obtain [Eq. (1) in the main text]

$$I_{\rm sf}(q) = I_{\rm sf}^0 \left[\frac{\sin(qR) - qR\cos(qR)}{q^3R^3}\right]^2 + I_{\rm sf}^1 \left[\frac{(q^2R^2-3)\sin(qR) + 3qR\cos(qR)}{q^4R^4}\right]^2, \tag{57}$$

where the $I_{\rm sf}^k$ are constant prefactors

$$I_{\rm sf}^k = \frac{1}{2\pi}\frac{8\pi^3 b_{\rm H}^2}{V}\int_0^{2\pi}\left(G_k^{xx} + G_k^{yy}\cos^4\theta + G_k^{zz}\sin^2\theta\cos^2\theta - (G_k^{yz} + G_k^{zy})\sin\theta\cos^3\theta\right)\, d\theta. \tag{58}$$

The first term in Eq. (57) corresponds to the form factor of a uniformly magnetized sphere, and the second term is the first-order extension. The zero- and first-order coefficients $I_{\rm sf}^0$ and $I_{\rm sf}^1$, as functions of the correlation coefficients $\Gamma$, are given by

$$I_{\rm sf}^0 = \frac{9V_{\rm s}^2 b_{\rm H}^2}{8V}\left(8\Gamma_0^{xx} + 3\Gamma_0^{yy} + \Gamma_0^{zz}\right), \tag{59}$$

$$I_{\rm sf}^1 = \frac{9V_{\rm s}^2 R^2 b_{\rm H}^2}{16V}\left(8\Gamma_{1,yy}^{xx} + 8\Gamma_{1,zz}^{xx} + \Gamma_{1,yy}^{yy} + 5\Gamma_{1,zz}^{yy} + \Gamma_{1,yy}^{zz} + \Gamma_{1,zz}^{zz} - 2\Gamma_{1,yz}^{yz} - 2\Gamma_{1,zy}^{yz}\right). \tag{60}$$

In the perfectly saturated state, the higher-order coefficients in Eq. (57) vanish and the remaining zeroth-order term is given by:

$$I_{\rm sf}(q; B_0 \to \infty) = I_{\rm sf}^{0,\rm sat} g_0(qR) = I_{\rm sf}^{0,\rm sat}\left[\frac{j(qR)}{qR}\right]^2. \tag{61}$$

The corresponding spin-flip pair-distance distribution function $p_{\rm sf}(r)$ is then obtained from the spherical Hankel transform of $I_{\rm sf}(q)$ [Eq. (57)] as:

$$\begin{aligned} p_{\rm sf}(r) &= r^2\int_0^\infty I_{\rm sf}(q) j_0(qr) q^2 dq \\ &= I_{\rm sf}^0 \frac{\pi r^2}{6R^3}\left[1 - \frac{3r}{4R} + \frac{r^3}{16R^3}\right] + I_{\rm sf}^1 \frac{\pi r^2}{10R^3}\left[1 - \frac{5r}{4R} + \frac{5r^3}{16R^3} - \frac{r^5}{32R^5}\right]. \end{aligned} \tag{62}$$

Here, the first term corresponds to the well-known pair-distance distribution function of a uniformly magnetized spherical nanoparticle, whereas the second term represents the first-order extension, with the ability to describe

vortex-like spin textures. For completeness, we remind the reader that the general boundary conditions for the pair-distance distribution function Eq. (62) in the case of objects of finite size are given by:

$$p_{\mathrm{sf}}(0) = 0, \qquad p_{\mathrm{sf}}(2R) = 0, \tag{63}$$

$$\left.\frac{dp_{\mathrm{sf}}}{dr}\right|_{r=0} = 0, \qquad \left.\frac{dp_{\mathrm{sf}}}{dr}\right|_{r=2R} = 0. \tag{64}$$

Figure 1 in the main paper displays the "phase diagram" for $I_{\mathrm{sf}}(q)$ and $p_{\mathrm{sf}}(r)$. Plotted are Eqs. (57) and (62) as functions of the ratio $I^1_{\mathrm{sf}}/I^0_{\mathrm{sf}}$. Already for $I^1_{\mathrm{sf}}/I^0_{\mathrm{sf}} > 1$, we find that $p_{\mathrm{sf}}(r)$ exhibits negative values above a certain distance $r$. The presence of negative values in the pair-distance distribution function (as well as in the correlation function) refers to antiparallel spin correlations. Therefore, such negative values are a strong indication for the presence of vortex-type spin structures. For even larger values of $I^1_{\mathrm{sf}}/I^0_{\mathrm{sf}}$, the distance distribution function reveals a damped oscillatory behavior with the zero crossing shifting to smaller $r$. This observation is accompanied by the appearance of a maximum in $I_{\mathrm{sf}}(q)$ at a certain momentum transfer $q$ that is different from $q = 0$. The transition point above which $I_{\mathrm{sf}}(q)$ shows a reduced behavior at $q = 0$ is given by a coefficient ratio $I^1_{\mathrm{sf}}/I^0_{\mathrm{sf}} > 5$.

We emphasize that in this formulation of the neutron-scattering observables it is only assumed that the magnetization vector field is of linear polynomial order. In the following, we derive analytical results for the specific case that this linear polynomial takes on the form of a vortex.

## IV. LINEAR THEORY FOR VORTEX SPIN STRUCTURES

For the particular case of a linear vortex profile, analytical expressions for $d\Sigma_{\mathrm{sf}}/d\Omega$ and chiral function $d\Sigma_{\chi}/d\Omega$ can be derived. For this, we assume that the magnetization vector field (for $r < R$) can be written as:

$$\mathbf{M}'(\mathbf{r}') = m_0\mathbf{e}'_z + m_1\mathbf{v}(\mathbf{r}'), \tag{65}$$

where $\mathbf{e}'_z = [0, 0, 1]$ is the unit vector in $z'$ direction, $\mathbf{v}(\mathbf{r}') = [-y', x', 0]$ is the linear vortex field, and $\mathbf{r}' = [x', y', z']$ is the position vector with reference to the local vortex frame. A positive value for $m_1$ indicates a counterclockwise (CCW) or right-handed sense of rotation, while a negative $m_1$ corresponds to a clockwise (CW) or left-handed sense of rotation. We note that for a micromagnetic Hamiltonian that contains the isotropic exchange interaction, magnetic anisotropy, and the Zeeman and magnetodipolar interaction there exists no preference for CCW or CW vortex rotation senses in the particles. CCW and CW vortices appear with equal probability so that the chiral function averages to zero (see below). By including the Dzyaloshinskii-Moriya interaction (DMI), which breaks space-inversion symmetry, chirality selection takes place and leads to a nonzero chiral function [15]. Applying the Fourier differentiation theorem, we obtain the following expression for the Fourier transform of the above local magnetization vector field:

$$\widetilde{\mathbf{M}}'(\mathbf{q}') = [-\mathrm{i}m_1\partial_{q_y}\widetilde{S}(q'),\ \mathrm{i}m_1\partial_{q'_x}\widetilde{S}(q'),\ m_0\widetilde{S}(q)], \tag{66}$$

where $\widetilde{S}$ denotes the spherical form-factor function

$$\widetilde{S}(q) = \frac{3V_{\mathrm{s}}}{(2\pi)^{3/2}}\frac{\sin(qR) - qR\cos(qR)}{q^3R^3}. \tag{67}$$

Using the chain rule we find:

$$\widetilde{\mathbf{M}}'(\mathbf{q}') = [-\mathrm{i}m_1\hat{q}'_yS'(q),\ \mathrm{i}m_1\hat{q}'_xS'(q'),\ m_0S(q')] \tag{68}$$

with

$$\widetilde{S}'(q) = \frac{d\widetilde{S}}{dq} = \frac{3V_{\mathrm{s}}}{(2\pi)^{3/2}}\frac{(q^2R^2 - 3)\sin(qR) + 3qR\cos(qR)}{q^4R^4}, \tag{69}$$

and $\hat{q}_\nu = q_\nu/q$ denotes the normalized Fourier space coordinates. We assume a dilute assembly of spherical nanoparticles with randomly-distributed orientations of the magnetocrystalline anisotropy. In this case, the magnetization vector field in the local particle frame [Eq. (65)] needs to be transformed into the global laboratory frame of reference by a $zy$ rotation matrix $\mathbf{R}(\alpha, \beta) = \mathbf{R}_z(\beta) \cdot \mathbf{R}_y(\alpha)$, where $\alpha$ is the polar angle and $\beta$ the azimuth angle. Such a rotation transformation is invariant when going from real space to Fourier space, which is why the transformation of the magnetization in Fourier space is transformed as:

$$\widetilde{\mathbf{M}}(\mathbf{q}; \alpha, \beta) = \mathbf{R}(\alpha, \beta) \cdot \widetilde{\mathbf{M}}'\left(\mathbf{R}^T(\alpha, \beta) \cdot \mathbf{q}\right). \tag{70}$$

Using the following definition of the correlation matrix of the Fourier magnetization vector field,

$$\widetilde{\Gamma}^{\iota\kappa}(\mathbf{q}) = \left[\widetilde{M}^{\iota}(\mathbf{q})\right]\left[\widetilde{M}^{\kappa}(\mathbf{q})\right]^*, \tag{71}$$

and by projection into the detector plane $\mathbf{q} = [0, q\sin\theta, q\cos\theta]$, the spin-flip SANS cross section $\frac{d\Sigma_{\mathrm{sf}}}{d\Omega}(q,\theta;\alpha,\beta)$ and the chiral function $\frac{d\Sigma_{\chi}}{d\Omega}(q,\theta;\alpha,\beta)$ corresponding to a single nanoparticle with vortex orientation $(\alpha,\beta)$ are written as (see also [8]):

$$\frac{d\Sigma_{\mathrm{sf}}}{d\Omega}(q,\theta;\alpha,\beta) = K\left[\widetilde{\Gamma}^{xx} + \widetilde{\Gamma}^{yy}\cos^4\theta + \widetilde{\Gamma}^{zz}\sin^2\theta\cos^2\theta - (\widetilde{\Gamma}^{yz} + \widetilde{\Gamma}^{zy})\sin\theta\cos^3\theta\right], \tag{72}$$

$$\frac{d\Sigma_{\chi}}{d\Omega}(q,\theta;\alpha,\beta) = K\left[(\widetilde{\Gamma}^{xy} - \widetilde{\Gamma}^{yx})\cos^2\theta + (\widetilde{\Gamma}^{xz} - \widetilde{\Gamma}^{zx})\sin\theta\cos\theta\right]. \tag{73}$$

In the MNPSE method, we define the ensemble-averaged (dilute) SANS cross sections as:

$$\left\langle \frac{d\Sigma_{\mathrm{sf},\chi}}{d\Omega} \right\rangle = \frac{1}{2}\int_0^{4\pi}\left[\frac{d\Sigma^{\mathrm{CCW}}_{\mathrm{sf},\chi}}{d\Omega} + \frac{d\Sigma^{\mathrm{CW}}_{\mathrm{sf},\chi}}{d\Omega}\right]\psi(\alpha,\beta)d\Upsilon \tag{74}$$

where $d\Upsilon = \sin\alpha d\alpha d\beta$ is the solid-angle differential, and $\frac{d\Sigma^{\mathrm{CCW}}_{\mathrm{sf},\chi}}{d\Omega}(\mathbf{q};\alpha,\beta)$ and $\frac{d\Sigma^{\mathrm{CW}}_{\mathrm{sf},\chi}}{d\Omega}(\mathbf{q};\alpha,\beta)$ are the SANS cross sections referring to two nanoparticles with the same orientation $(\alpha,\beta)$, but opposite senses of vortex rotation ($m_1^{\mathrm{CCW}} = -m_1^{\mathrm{CW}}$). The function $\psi(\alpha,\beta)$ is a field-dependent probability distribution modelling the orientation of both the CCW and CW vortex rotation axes (no distinction between the different polarities). For simplicity, we assume a uniform distribution $\psi_{\mathrm{u}}$ on the spherical surface, which is limited by a field-dependent conical opening angle $0° \leq \alpha_{\mathrm{c}} \leq 90°$. The azimuthally-symmetric distribution function is then given by:

$$\psi_{\mathrm{u}}(\alpha,\beta) = \frac{\Theta(1-\alpha/\alpha_c)}{2\pi(1-\cos\alpha_c)}, \tag{75}$$

where $\Theta(\xi)$ is the Heaviside function. Finally, the resulting spin-flip SANS cross section and chiral function for a dilute ensemble of spherical nanoparticles with vortex type spin structures reads ($\mathbf{H}_0 \perp \mathbf{k}_0$):

$$\begin{aligned}\left\langle \frac{d\Sigma_{\mathrm{sf}}}{d\Omega} \right\rangle(q,\theta) = {} & \frac{W}{8}[m_0 f(qR)]^2 \times \left[12 - (\cos^2\alpha_{\mathrm{c}} + \cos\alpha_{\mathrm{c}})(3\cos^2(2\theta) + 2\cos(2\theta) + 3) + 4\cos(2\theta)\right] \\ & + \frac{W}{2}[m_1 R f'(qR)]^2 \times \left[3 - (2\cos^2\alpha_{\mathrm{c}} + 2\cos\alpha_{\mathrm{c}} - 1)\cos(2\theta)\right],\end{aligned} \tag{76}$$

$$\left\langle \frac{d\Sigma^{\mathrm{CCW,CW}}_{\chi}}{d\Omega} \right\rangle(q,\theta) = \pm W\left[m_0|m_1|Rf(qR)f'(qR)\cos\theta\right] \times \left[4 + \cos^2\alpha_{\mathrm{c}} + \cos\alpha_{\mathrm{c}} - 3(\cos^2\alpha_{\mathrm{c}} + \cos\alpha_{\mathrm{c}})\cos^2\theta\right], \tag{77}$$

where $W = 3V_{\mathrm{s}}^2 b_{\mathrm{H}}^2/V$. The "+" sign in Eq. (77) stands for CCW and the "−" sign for CW vortex rotations. Equations (76) and (77) are displayed in Fig. 2 in the main paper. When no chirality selection takes place, then it follows that:

$$\left\langle \frac{d\Sigma_{\chi}}{d\Omega} \right\rangle = \frac{1}{2}\left[\left\langle \frac{d\Sigma^{\mathrm{CCW}}_{\chi}}{d\Omega} \right\rangle + \left\langle \frac{d\Sigma^{\mathrm{CW}}_{\chi}}{d\Omega} \right\rangle\right] = 0. \tag{78}$$

The azimuthally-averaged spin-flip SANS cross section then equals:

$$\begin{aligned}\langle I_{\mathrm{sf}}\rangle(q) &= \frac{1}{2\pi}\int_0^{2\pi}\left\langle \frac{d\Sigma_{\mathrm{sf}}}{d\Omega} \right\rangle(q,\theta)d\theta \\ &= \frac{3W}{16}\left([m_0 f(qR)]^2(8 - 3\cos^2\alpha_{\mathrm{c}} - 3\cos\alpha_{\mathrm{c}}) + 8[m_1 R f'(qR)]^2\right).\end{aligned} \tag{79}$$

Comparing this expression to Eq. (57) we find:

$$I^0_{\mathrm{sf}} = \frac{3W}{16}m_0^2(8 - 3\cos^2\alpha_{\mathrm{c}} - 3\cos\alpha_{\mathrm{c}}), \tag{80}$$

$$I^1_{\mathrm{sf}} = \frac{3W}{16}8m_1^2R^2, \tag{81}$$

$$\iota = \frac{I^1_{\mathrm{sf}}}{I^0_{\mathrm{sf}}} = \frac{8m_1^2R^2}{m_0^2(8 - 3\cos^2\alpha_{\mathrm{c}} - 3\cos\alpha_{\mathrm{c}})}. \tag{82}$$

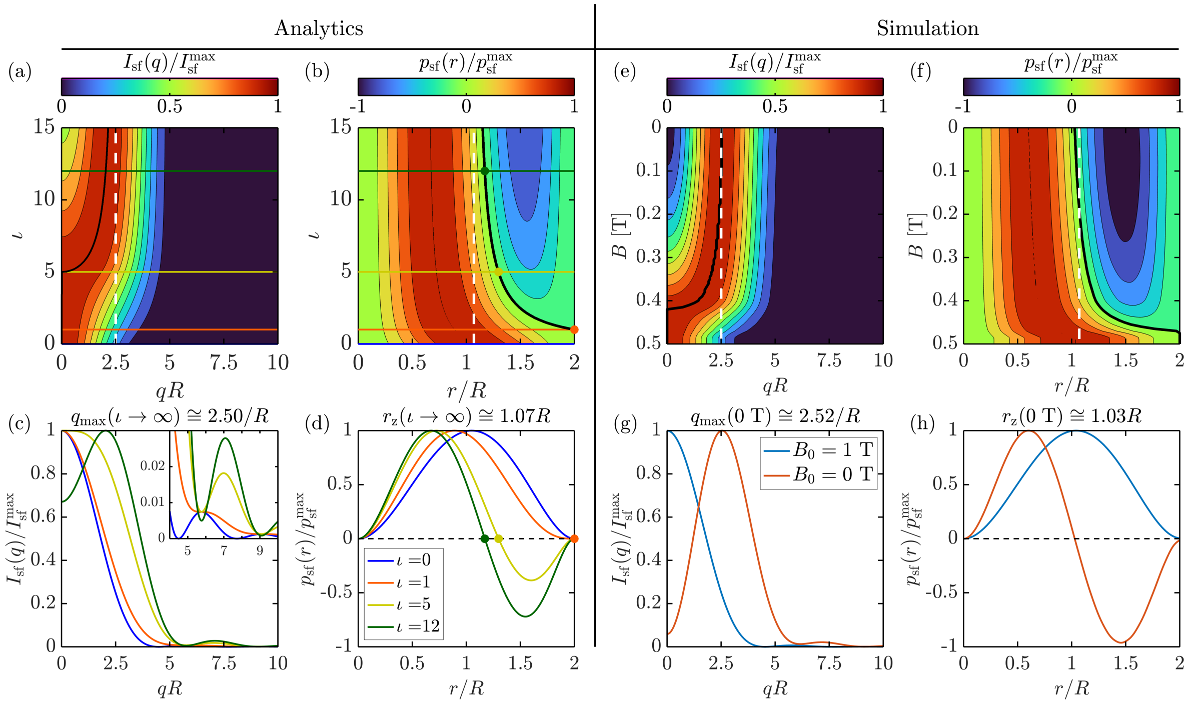


FIG. 6. Same as Fig. 1 in the main paper, but for a uniaxial particle anisotropy (1600 random orientations). "Phase diagram" for the azimuthally-averaged spin flip SANS cross section $I_{sf}(q)$ [Eq. (57)] and for the spin-flip pair-distance distribution function $p_{sf}(r)$ [Eq. (62)] within the limits of the first-order magnetization model. The left panel shows the analytical results, while the right panel features the corresponding results of the micromagnetic simulations. The ratio $\iota$ of the zero-order coefficient $I_{sf}^0$ and the first-order coefficient $I_{sf}^1$ determines the appearance of vortex-type spin structures. Field ($B_0 = \mu_0 H_0$) variations in the simulations correspond to $\iota$ variations in the analytical part (zero field: $\iota \to \infty$; saturation: $\iota \to 0$). (a) Color-coded plot of the normalized $I_{sf}(q)$ as a function of $\iota = I_{sf}^1/I_{sf}^0$ and $qR$. The black solid line in (a) describes the shift of the maximum in $I_{sf}(q)$ towards $q_{max} \cong 2.50/R$ [white dashed line, compare (e)]. (b) Normalized $p_{sf}(r)$ as a function of $\iota$ and $r/R$. The black solid line in (b) describes the shift of the zero in $p_{sf}(r)$ towards $r_z \cong 1.07R$ [white dashed line, compare (f)]. (c) Normalized $I_{sf}(qR)$ and (d) normalized $p_{sf}(r/R)$ for different $\iota$ [see inset in (d)]; the inset in (c) displays $I_{sf}(q)/I_{sf}^{max}$ for $4 < qR < 10$. The colored horizontal lines in (a) and (b) correspond, respectively, to the curves in (c) and (d).

## V. UNIAXIAL VERSUS CUBIC RANDOM ANISOTROPY

The micromagnetic simulation results that are reported in the main paper were carried out using the materials parameters of iron, which possesses a cubic magnetocrystalline anisotropy. Figures 6−9 show the results when a random uniaxial anisotropy is used in the simulations, instead of a random cubic anisotropy. More specifically, the following expression for the magnetic anisotropy energy has been used [replacing Eq. (14)]:

$$E_{ani} = -K_{u1} \int (\mathbf{e}_A \cdot \mathbf{m})^2 \, dV, \tag{83}$$

where $K_{u1} = +4.7 \times 10^4$ J/m$^3$ denotes the first-order uniaxial anisotropy constant, and $\mathbf{e}_A$ is a unit vector specifying the local random easy-axis direction of a particle. Comparing Figs. 6 and 7 with Figs. 1 and 2 in the main paper, and likewise Figs. 2 and 3 with Figs. 8 and 9, see that the behavior is qualitatively and quantitatively very similar.

We acknowledge financial support from the National Research Fund of Luxembourg (AFR Grant No. 15639149, CORE Grant DeQuSky, and PRIDE MASSENA Grant).

[1] D. Honecker, A. Ferdinand, F. Döbrich, C. D. Dewhurst, A. Wiedenmann, C. Gómez-Polo, K. Suzuki, and A. Michels, Eur. Phys. J. B **76**, 209 (2010).

[2] K. L. Krycka, J. A. Borchers, R. A. Booth, Y. Ijiri, K. Hasz, J. J. Rhyne, and S. A. Majetich, Phys. Rev. Lett. **113**, 147203 (2014).

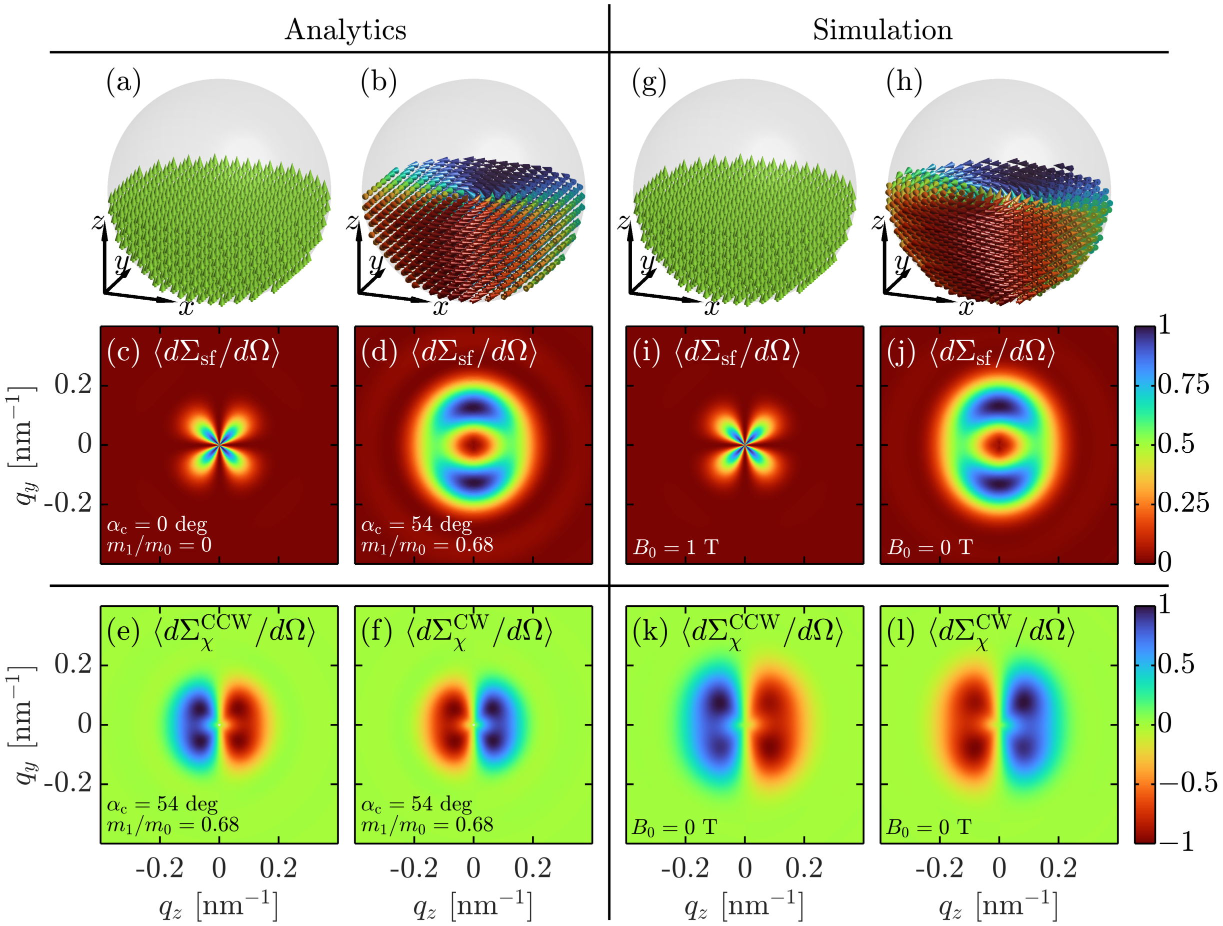


FIG. 7. Same as Fig. 2 in the main paper, but for a uniaxial particle anisotropy (1600 random orientations). Illustration of the 2D (normalized) spin-flip SANS cross section and chiral function computed from Eqs. (76) and (77) reflecting the saturation and remanence cases (particle size: $D = 2R = 40\,\mathrm{nm}$) (linear color scale). (a,b) and (g,h) show snapshots of the underlying real-space spin structures. The left panel shows the analytical results, while the right panel features the results of the micromagnetic simulations. The incoming neutron beam is perpendicular to the applied magnetic field $\mathbf{H}_0 \parallel \mathbf{e}_z$ ($B_0 = \mu_0 H_0$). The maximum of the spots in (d) and (j) are found at $q_{y,\max} \cong 2.50/R$. (e,f) and (k,l) display the respective chiral functions in the remanent state for counterclockwise (CCW) and clockwise (CW) vortex rotations. Note that the specific values for $\alpha_c = 54°$ and for the ratio $m_1/m_0 = 0.68$ in (d) are based on a fit of the analytical function [Eq. (76)] to the 2D simulation data shown in (j).


[3] D. Zákutná, D. Nižňanský, L. C. Barnsley, E. Babcock, Z. Salhi, A. Feoktystov, D. Honecker, and S. Disch, Phys. Rev. X **10**, 031019 (2020).
[4] C. Kons, K. L. Krycka, J. Robles, N. Ntallis, M. Pereiro, M.-H. Phan, H. Srikanth, J. A. Borchers, and D. A. Arena, ACS Appl. Nano Mater. **6**, 10986 (2023).
[5] V. Ukleev, F. Ajejas, A. Devishvili, A. Vorobiev, N.-J. Steinke, R. Cubitt, C. Luo, R.-M. Abrudan, F. Radu, V. Cros, N. Reyren, and J. S. White, STAM Methods **25**, 2315015 (2024).
[6] A. Michels, *Magnetic Small-Angle Neutron Scattering: A Probe for Mesoscale Magnetism Analysis* (Oxford University Press, Oxford, 2021).
[7] M. P. Adams, A. Michels, and H. Kachkachi, J. Appl. Cryst. **55**, 1488 (2022).
[8] M. P. Adams, E. P. Sinaga, H. Kachkachi, and A. Michels, Phys. Rev. B **109**, 024429 (2024).
[9] A. Vansteenkiste, J. Leliaert, M. Dvornik, M. Helsen, F. Garcia-Sanchez, and B. Van Waeyenberge, AIP Advances **4**, 107133 (2014).
[10] J. Leliaert, M. Dvornik, J. Mulkers, J. De Clercq, M. V. Milošević, and B. Van Waeyenberge, J. Phys. D: Appl. Phys. **51**, 123002 (2018).
[11] W. F. Brown Jr., *Micromagnetics* (Interscience Publishers, New York, 1963).
[12] In the simulations, $\mathbf{c}_1$ is a random unit vector that is generated using two random angles. A second random unit vector, say $\mathbf{b}$, is generated by another set of random angles, such that $\mathbf{c}_2 = (\mathbf{c}_1 \times \mathbf{b})/|\mathbf{c}_1 \times \mathbf{b}|$ and $\mathbf{c}_3 = \mathbf{c}_1 \times \mathbf{c}_2$.
[13] This follows from the fact that the SANS cross section is a real-valued quantity.

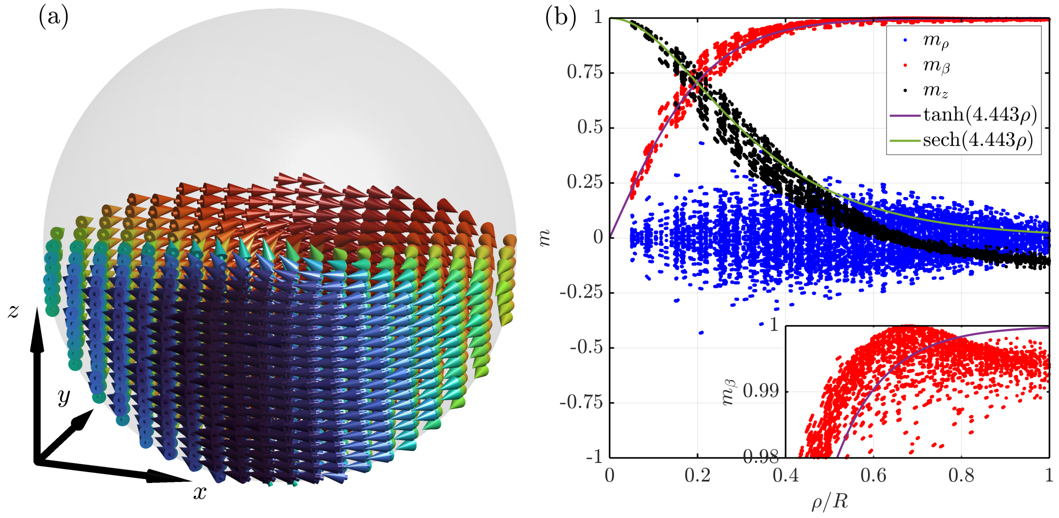


FIG. 8. Same as Fig. 2, but for a uniaxial particle anisotropy (1600 random orientations).

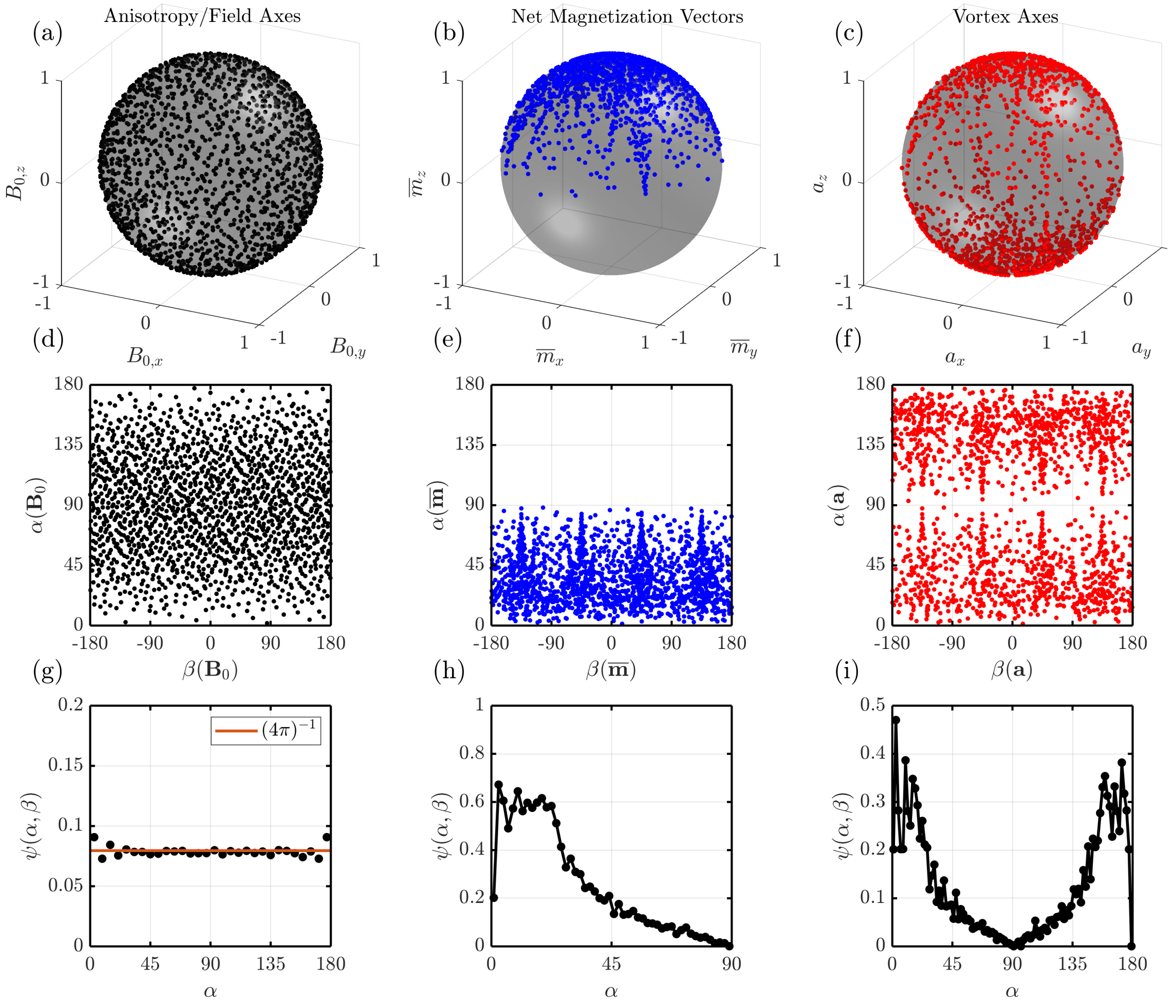


FIG. 9. Same as Fig. 3, but for a uniaxial particle anisotropy (1600 random orientations).

[14] M. P. Adams, E. P. Sinaga, and A. Michels, IUCrJ **10**, 261 (2023).

[15] E. P. Sinaga, M. P. Adams, E. H. Hasdeo, and A. Michels, (2024), arXiv:2402.00558 [cond-mat.mes-hall].
